# Supplementary material for: Black-box Importance Sampling
Source: arXiv:1610.05247 source file (2016-10-17)
Supplement: Supplementary file 1 [file appendix.pdf]

---

# Black-Box Importance Sampling

---

**Anonymous Author 1**  
Unknown Institution 1

**Anonymous Author 2**  
Unknown Institution 2

**Anonymous Author 3**  
Unknown Institution 3

## 1 Kernelized Stein Discrepancy and MMD

Given RKHS  $\mathcal{H}$  with kernel  $k(x, x')$ , the maximum mean discrepancy (MMD) between two distributions with density  $p(x)$  and  $q(x)$  is defined as

$$\text{MMD}_{\mathcal{H}}(q, p) = \max_{f \in \mathcal{H}} \{ \mathbb{E}_q f - \mathbb{E}_p f \quad \text{s.t.} \quad \|f\|_{\mathcal{H}} \leq 1 \},$$

which can be shown to be equivalent to

$$\text{MMD}_{\mathcal{H}}(q, p) = \mathbb{E}_{x, x' \sim p} [k(x, x')] - 2\mathbb{E}_{x \sim p; y \sim q} [k(x, y)] + \mathbb{E}_{y, y' \sim q} [k(y, y')].$$

We show that kernelized discrepancy  $\mathbb{S}(q, p)$  is equivalent to  $\text{MMD}_{\mathcal{H}_p}(q, p)$ , equipped with the  $p$ -Steinized kernel  $k_p(x, x')$ .

**Proposition 1.1.** *Assume (3) is true, we have*

$$\mathbb{S}(q, p) = \text{MMD}_{\mathcal{H}_p}(q, p).$$

*Proof.* Simply note that  $\mathbb{E}_{x' \sim p} [k_p(x, x')] = 0$  for any  $x$ , we have

$$\text{MMD}_{\mathcal{H}_p}(q, p) = \mathbb{E}_{x, x' \sim q} [k_p(x, x')] = \mathbb{S}(q, p).$$

□

Similarly, we also have

$$\begin{aligned} \mathbb{S}(\{x_i, w_i\}_{i=1}^n, p) &= \text{MMD}_{\mathcal{H}_p}(\{x_i, w_i\}, p) \\ &:= \max_{f \in \mathcal{H}} \left\{ \sum_i w_i f(x_i) - \mathbb{E}_p f \quad \text{s.t.} \quad \|f\|_{\mathcal{H}} \leq 1 \right\}. \end{aligned}$$

*Proof of Proposition 3.1.* Let  $\tilde{h}(x) = h(x) - \mathbb{E}_p h$ , we have

$$\begin{aligned} \left| \sum_i w_i \tilde{h}(x_i) \right| &= \left| \sum_i w_i \langle \tilde{h}, k_p(\cdot, x_i) \rangle_{\mathcal{H}_p} \right| \\ &= \left| \langle \tilde{h}, \sum_i w_i k_p(\cdot, x_i) \rangle_{\mathcal{H}_p} \right| \\ &\leq \|\tilde{h}\|_{\mathcal{H}_p} \cdot \left\| \sum_i w_i k_p(\cdot, x_i) \right\|_{\mathcal{H}_p} \\ &= \|\tilde{h}\|_{\mathcal{H}_p} \cdot \sqrt{\mathbb{S}(\{w_i, x_i\}, p)}. \end{aligned}$$

where we used Cauchy-Schwarz inequality and the fact that  $\left\| \sum_i w_i k_p(\cdot, x_i) \right\|_{\mathcal{H}_p}^2 = \sum_{i,j} w_i w_j k_p(x_i, x_j) = \mathbb{S}(\{w_i, x_i\}, p)$ . □

## 2 Convergence Rate

We consider the error rate of our estimator  $\sum_i \hat{w}_i(\mathbf{x})h(x_i)$  with  $\{\hat{w}_i(\mathbf{x})\}$  given by the optimization in (6), under the assumption that  $\mathbf{x} = \{x_i\}_{i=1}^n$  is i.i.d. drawn from an (unknown) distribution  $q(x)$ . Based on the bound in Proposition (3.1), we can establish an error rate  $\mathcal{O}(n^{-\delta})$  by finding a set of oracle “reference weights”  $\{w_{*i}(\mathbf{x})\}$ , as a function of  $\mathbf{x}$ , such that  $\mathbb{S}(\{x_i, w_{*i}(\mathbf{x})\}, p) = \mathcal{O}(n^{-2\delta})$ , because

$$|\sum_i \hat{w}_i(\mathbf{x})h(x_i) - \mathbb{E}_p h| \leq C_h \cdot \sqrt{\mathbb{S}(\{\hat{w}_i(\mathbf{x}), x_i\}, p)} \leq C_h \cdot \sqrt{\mathbb{S}(\{w_{*i}(\mathbf{x}), x_i\}, p)} = \mathcal{O}(n^{-\delta}),$$

where  $C_h = \|h - \mathbb{E}_p h\|_{\mathcal{H}_p}$ . This idea of using reference weights has been used in Briol et al. [2015a] to study the convergence rate of Bayesian Monte Carlo.

Section 2.1 proves the  $\mathcal{O}(n^{-1/2})$  rate using the typical importance sampling weights as the reference weight. Section 2.2 proves a better  $\mathcal{O}(n^{-1/2})$  rate by using a reference weight based on a control variates method constructed with an orthogonal basis estimator.

### 2.1 $\mathcal{O}(n^{-1/2})$ Rate

We use the typical importance sampling weight as a reference weight and establish  $\mathcal{O}(n^{-1/2})$  rate on the error of our estimator.

**Assumption 2.1.** Assume  $p(x)/q(x) > 0$  for  $\forall x \in \mathcal{X}$  and  $\mathbb{E}_{x \sim q}[(\frac{p(x)}{q(x)})^2] < \infty$ ,  $\mathbb{E}_{x \sim q}(|\frac{p(x)}{q(x)} k_p(x, x)|) < \infty$ , and  $\mathbb{E}_{x, x' \sim q}[(\frac{p(x)p(x')}{q(x)q(x')} k_p(x, x'))^2] < \infty$ .

**Lemma 2.2.** Assume  $\{x_i\}_{i=1}^n$  is i.i.d. drawn from  $q(x)$

$$w_i^* = \frac{1}{Z} p(x_i)/q(x_i), \quad Z = \sum_i p(x_i)/q(x_i),$$

then under Assumption 2.1 we have

$$\mathbb{S}(\{w_i^*, x_i\}, p) = \mathcal{O}(n^{-1}).$$

*Proof.* Define  $v_i^*(x_i) = \frac{1}{n} p(x_i)/q(x_i)$ , and

$$\mathbb{S}(\{v_i^*, x_i\}, p) = \frac{1}{n^2} \sum_{ij} \frac{p(x_i)}{q(x_i)} \frac{p(x_j)}{q(x_j)} k_p(x_i, x_j),$$

then  $\mathbb{S}(\{v_i^*, x_i\}, p)$  is a degenerate V-statistic since by (3) we have

$$\mathbb{E}_{x' \sim q}[\frac{p(x)}{q(x)} \frac{p(x')}{q(x')} k_p(x', x')] = \frac{p(x)}{q(x)} \mathbb{E}_{x' \sim p}[k_p(x_i, x_j)] = 0, \quad \forall x \in \mathcal{X}$$

then we have [see e.g., Lee, 1990]

$$\mathbb{S}(\{v_i^*, x_i\}, p) = \mathcal{O}(n^{-1}).$$

In addition, note that  $\sum_{i=1}^n v_i^* = 1 + \mathcal{O}(n^{-1/2})$ , we have

$$\mathbb{S}(\{w_i^*, x_i\}, p) = \frac{\mathbb{S}(\{v_i^*, x_i\}, p)}{(\sum_i v_i^*)^2} = \mathcal{O}(n^{-1}).$$

□

**Theorem 2.3.** Assume  $\{x_i\}$  is i.i.d. drawn from  $q(x)$ , and  $\{\hat{w}_i(\mathbf{x})\}$  is given by (6), then under Assumption 2.1, we have

$$\sum_{i=1}^n \hat{w}_i(\mathbf{x})h(x_i) - \mathbb{E}_p h = \mathcal{O}(n^{-1/2}).$$

*Proof.* Simply note that

$$\mathbb{S}(\{\hat{w}_i, x_i\}_{i=1}^n, p) \leq \mathbb{S}(\{w_i^*, x_i\}_{i=1}^n, p) = \mathcal{O}(n^{-1}),$$

and combining with Proposition 3.1 gives the result. □

## 2.2 $\mathcal{O}(n^{-1/2})$ Rate

We prove Theorem 3.3 that shows an  $\mathcal{O}(n^{-1/2})$  rate for our estimator. Our method is based on constructing a reference weight by using a two-fold control variate method based on the first  $L$  orthogonal eigenfunctions  $\{\phi_\ell\}$  of kernel  $k_p(x, x')$ .

We first re-state the assumptions made in Theorem 3.3.

**Assumption 2.4.** 1. Assume  $k_p(x, x')$  has the following eigen-decomposition

$$k_p(x, x') = \sum_{\ell} \lambda_{\ell} \phi_{\ell}(x) \phi_{\ell}(x'),$$

where  $\lambda_{\ell}$  are the positive eigenvalues sorted in non-increasing order, and  $\phi_{\ell}$  are the eigenfunctions orthonormal w.r.t. distribution  $p(x)$ , that is,

$$\mathbb{E}_p[\phi_{\ell} \phi_{\ell'}] \stackrel{\text{def}}{=} \int p(x) \phi_{\ell}(x) \phi_{\ell'}(x) dx = \mathbb{I}[\ell = \ell'].$$

2.  $\text{trace}(k_p(x, x')) = \sum_{\ell=1}^{\infty} \lambda_{\ell} < \infty$ .

3.  $\text{var}_{x \sim q}[w_*(x)^2 \phi_{\ell}(x) \phi_{\ell'}(x)] \leq M$  for all  $\ell$  and  $\ell'$ , where  $w_*(x) = p(x)/q(x)$ .

4.  $|\phi_{\ell}(x)|^2 \leq M_2$ , and  $w_*(x) \stackrel{\text{def}}{=} p(x)/q(x) \leq M_3$  for any  $x \in \mathcal{X}$ .

The following is an expended version of Theorem 3.3.

**Theorem 2.5.** Assume  $\{x_i\}_{i=1}^n$  is i.i.d. drawn from  $q(x)$ , and  $\hat{w}_i$  is calculated by

$$\hat{\mathbf{w}} = \arg \min_{\mathbf{w}} \mathbf{w} \mathbf{K}_p \mathbf{w}, \quad \text{s.t.} \sum_i w_i = 1, \quad w_i \geq 0,$$

and  $h - \mathbb{E}_p h \in \mathcal{H}_p$ . Under Assumption 2.4, we have

$$\mathbb{E}_{\mathbf{x} \sim q}(|\sum_i \hat{w}_i h(x_i) - \mathbb{E}_p h|^2) = \mathcal{O}(\frac{1}{n} \gamma(n)),$$

$$\text{where} \quad \gamma(n) = \min_{L \in \mathbb{N}^+} \left\{ \frac{M_3}{2} \mathbb{R}(L) + \frac{M_4}{2} \frac{L}{n} + M_f n(n+2) \exp(-\frac{n}{L^2 M_0}) \right\},$$

where  $\mathbb{N}^+$  is the set of positive integers, and  $\mathbb{R}(L) = \sum_{\ell > L} \lambda_{\ell}$  is the residual of the spectrum, and  $M_4 = 2M_3 M \text{trace}(k_p)$ . and  $M_f = \text{trace}(k_p(x, x')) M_2$  and  $M_0 = \max(M_2^2 M_3, M_3^2 (M_2 M_3 + \sqrt{2})^2)$ .

**Remark** To see how Theorem 2.5 implies Theorem 3.3, we just need to observe that we obviously have  $\gamma(n) \geq 2M_3 \frac{b}{n}$ , and  $\gamma(n) = \mathcal{O}(1)$  by taking  $L = n^{1/4}$ .

Based on Proposition 3.1, to prove Theorem 2.5 we just need to show that for any  $\mathbf{x} = \{x_i\}_{i=1}^n$ , there exists a set of positive and normalized weights  $\{w_i^+(\mathbf{x})\}$ , as a function of  $\mathbf{x}$ , such that

$$\mathbb{E}_{\mathbf{x} \sim q}[\mathbb{S}(\{w_i^+(\mathbf{x}), x_i\}, p)] = \mathcal{O}(\frac{\gamma(n)}{n}).$$

In the sequel, we construct such a weight based on a control variates method which uses the top eigenfunctions  $\phi_{\ell}$  as the control variates. Our proof includes the following steps:

1. Step 1: Construct a control variate estimator based on the orthogonal eigenfunction basis, and obtain the corresponding weights  $\{w_i(\mathbf{x})\}$ .
2. Step 2: Bound  $\mathbb{E}_{\mathbf{x} \sim q}[\mathbb{S}(\{w_i(\mathbf{x}), x_i\}, p)]$ .
3. Step 3. Construct a set of positive and normalized weights by  $w_i^+(\mathbf{x}) = \frac{\max(0, w_i(\mathbf{x}))}{\sum_i \max(0, w_i(\mathbf{x}))}$ , and establish the corresponding bound.

*Proof of Theorem 2.5.* Combine the bound in Lemma 2.7 and Lemma 2.9 below.  $\square$

We note that the idea of using reference weights was used in Briol et al. [2015a] to establish the convergence rate of Bayesian Monte Carlo. Related results is also presented in Bach [2015]. The main additional challenge in our case is to meet the non-negative and normalization constraint (Step 3); this is achieved by showing that the  $\{w_i(\mathbf{x})\}$  constructed in Step 2 is non-negative with high probability, and their sum approaches to one when  $n$  is large, and hence  $\{w_i^+(\mathbf{x})\}$  is not significantly different from  $\{w_i(\mathbf{x})\}$ .

Note that if we discard the non-negative and normalization constraint (Step 3), the error bound would be  $\mathcal{O}(\gamma_0(n)n^{-1})$ , where

$$\gamma_0(n) = \min_{L \in \mathbb{N}^+} \{2M_3\mathbb{R}(L) + 2M_4\frac{L}{n}\},$$

as implied by Lemma 2.7. Therefore, the third term in  $\gamma(n)$  is the cost to pay for enforcing the constraints. However, this additional term does not influence the rate significantly once  $\mathbb{R}(L) = \sum_{\ell > L} \lambda_\ell$  decays sufficiently fast. For example, when  $\mathbb{R}(L) = \mathcal{O}(L^{-\alpha})$  where  $\alpha > 1$ , both  $\gamma(n)$  and  $\gamma_0(n)$  equal  $\mathcal{O}(n^{-1+1/(\alpha+1)})$ ; when  $\mathbb{R}(L) = \mathcal{O}(\exp(-\alpha L))$  with  $\alpha > 0$ , both  $\gamma(n)$  and  $\gamma_0(n)$  equal  $\mathcal{O}(\frac{\log n}{n})$ . An open question is to derive upper bounds for the decay of eigenvalues  $\mathbb{R}(L)$  for given  $p$  and  $k(x, x')$ , so that actual rates can be determined.

### Step 1: Constructing the weights

We first construct a set of unnormalized, potentially negative reference weights, by using a two-fold control variates method based on the orthogonal eigenfunctions  $\{\phi_\ell\}$  of kernel  $k_p(x, x')$ . Assume  $n$  is an even number, and we partition the data  $\{x_i\}_{i=1}^n$  into two parts  $\mathcal{D}_0 = \{1, \dots, \frac{n}{2}\}$  and  $\mathcal{D}_1 = \{\frac{n}{2} + 1, \dots, n\}$ . For any  $h \in \mathcal{H}_p$ , we have  $\mathbb{E}_p h = 0$  by (3), and

$$h(x) = \sum_{\ell=1}^{\infty} \beta_\ell \phi_\ell(x), \quad \beta_\ell = \mathbb{E}_{x \sim p}[h(x)\phi_\ell(x)].$$

We now construct an orthogonal series estimator  $\hat{h}(x)$  for  $h(x)$  based on  $\mathbf{x}_{\mathcal{D}_0}$ ,

$$\hat{h}_{\mathcal{D}_0}(x) = \sum_{\ell=1}^L \hat{\beta}_{\ell,0} \phi_\ell(x), \quad \text{where} \quad \hat{\beta}_{\ell,0} = \frac{2}{n} \sum_{i \in \mathcal{D}_0} h(x_i) \phi_\ell(x_i) \frac{p(x_i)}{q(x_i)}, \quad (1)$$

where we approximate  $\beta_\ell$  with an unbiased estimator  $\hat{\beta}_{\ell,0}$  since

$$\mathbb{E}_{x \sim q}[\hat{\beta}_{\ell,0}] = \mathbb{E}_{x \sim q}[h(x)\phi_\ell(x) \frac{p(x)}{q(x)}] = \int p(x)h(x)\phi_\ell(x)dx = \beta_\ell.$$

We also truncate at the  $L$ th basis functions to keep  $\hat{h}_{\mathcal{D}_0}(x)$  a smooth function, as what is typically done in orthogonal basis estimators. We will discuss the choice of  $L$  later. Based on this we define a control variates estimator:

$$\hat{Z}_0[h] = \frac{2}{n} \sum_{i \in \mathcal{D}_1} [w_*(x_i)(h(x_i) - \hat{h}_{\mathcal{D}_0}(x_i))],$$

which gives an unbiased estimator for  $\mathbb{E}_p h = 0$  because

$$\mathbb{E}_{\mathbf{x} \sim q}(\hat{Z}_0[h]) = \int q(x) \frac{p(x)}{q(x)} (h(x) - \hat{h}_{\mathcal{D}_0}(x)) dx = \mathbb{E}_{x \sim p} h - \mathbb{E}_{\mathbf{x}_{\mathcal{D}_0} \sim q} [\mathbb{E}_{x \sim p}[\hat{h}_{\mathcal{D}_0}(x) \mid \mathbf{x}_{\mathcal{D}_0}]] = 0,$$

where the last step is because  $\mathbb{E}_{x \sim p}[\hat{h}_{\mathcal{D}_0}(x) \mid \mathbf{x}_{\mathcal{D}_0}] = \sum_{\ell=1}^L \hat{\beta}_{\ell,0} \mathbb{E}_{x \sim p}[\phi_\ell(x)] = 0$ . Switching  $\mathcal{D}_0$  and  $\mathcal{D}_1$ , we get another estimator

$$\hat{Z}_1[h] = \frac{2}{n} \sum_{i \in \mathcal{D}_0} [w_*(x_i)(h(x_i) - \hat{h}_{\mathcal{D}_1}(x_i))].$$

Averaging them gives

$$\hat{Z}[h] = \frac{\hat{Z}_0[h] + \hat{Z}_1[h]}{2}.$$

**Lemma 2.6.** Given  $\hat{Z}[h]$  defined as above, for any  $h \in \mathcal{H}_p$ , we have

$$\hat{Z}[h] = \sum_{i=1}^n w_i(\mathbf{x})h(x_i), \quad \text{with} \quad w_i(\mathbf{x}) = \begin{cases} \frac{1}{n}w_*(x_i) - \frac{2}{n^2} \sum_{j \in \mathcal{D}_1} w_*(x_i)w_*(x_j)k_L(x_j, x_i), & \forall i \in \mathcal{D}_0 \\ \frac{1}{n}w_*(x_i) - \frac{2}{n^2} \sum_{j \in \mathcal{D}_0} w_*(x_i)w_*(x_j)k_L(x_j, x_i), & \forall i \in \mathcal{D}_1 \end{cases}$$

where  $w_*(x) = p(x)/q(x)$  and  $k_L(x, x') = \sum_{\ell=1}^L \phi_\ell(x)\phi_\ell(x')$ .

*Proof.* We have

$$\begin{aligned} \hat{Z}_0[h] &= \frac{2}{n} \left[ \sum_{i \in \mathcal{D}_1} w_*(x_i)(h(x_i) - \hat{h}_{\mathcal{D}_0}(x_i)) \right] \\ &= \frac{2}{n} \left[ \sum_{i \in \mathcal{D}_1} w_*(x_i)(h(x_i) - \sum_{\ell=1}^L \hat{\beta}_{\ell,0} \phi_\ell(x)) \right] \\ &= \frac{2}{n} \left[ \sum_{i \in \mathcal{D}_1} w_*(x_i)(h(x_i) - \frac{2}{n} \sum_{\ell=1}^L \sum_{j \in \mathcal{D}_0} h(x_j)w_*(x_j)\phi_\ell(x_j)\phi_\ell(x_i)) \right] \\ &= \frac{2}{n} \sum_{i \in \mathcal{D}_1} w_*(x_i)h(x_i) - \frac{4}{n^2} \sum_{j \in \mathcal{D}_0} \sum_{i \in \mathcal{D}_1} h(x_j)w_*(x_j)w_*(x_i) \sum_{\ell=1}^L \phi_\ell(x_j)\phi_\ell(x_i) \\ &= \frac{2}{n} \sum_{i \in \mathcal{D}_1} w_*(x_i)h(x_i) - \frac{4}{n^2} \sum_{j \in \mathcal{D}_0} \sum_{i \in \mathcal{D}_1} h(x_j)w_*(x_j)w_*(x_i)k_L(x_i, x_j) \\ &\stackrel{\text{def}}{=} \sum_{i=1}^n w_{i,0}h(x_i), \end{aligned}$$

where

$$w_{i,0} = \begin{cases} -\frac{4}{n^2} \sum_{j \in \mathcal{D}_1} w_*(x_i)w_*(x_j)k_L(x_j, x_i) & \forall i \in \mathcal{D}_0 \\ \frac{2}{n}w_*(x_i) & \forall i \in \mathcal{D}_1 \end{cases} \quad (2)$$

We can derive the same result for  $\hat{Z}_1[h]$  and averaging them would gives the result.  $\square$

**Step 2: Calculating  $\mathbb{E}_{\mathbf{x} \sim q}(\mathbb{S}(\{x_i, w_i(\mathbf{x})\}, p))$**

**Lemma 2.7.** Under Assumption 2.4, for the weights  $\{w_i(\mathbf{x})\}$  defined in Lemma 2.6, we have

$$\mathbb{E}_{\mathbf{x} \sim q}[\mathbb{S}(\{x_i, w_i(\mathbf{x})\}, p)] \leq \frac{2}{n} [M_3 \mathbb{R}(L) + M_4 \frac{L}{n}]$$

where  $M_3$  is the upper bound of  $p(x)/q(x)$ ,  $\forall x \in \mathcal{X}$  and  $\mathbb{R}(L) = \sum_{\ell > L} \lambda_\ell$  and  $M_4 = 2M_3 \max_{\ell'} \{\sum_{\ell} \lambda_\ell \rho_{\ell\ell'}\} \leq 2M_3 M_{\text{trace}}(k_p)$ .

*Proof.* First, for any  $h \in \mathcal{H}_p$  (such that  $\mathbb{E}_p[h] = 0$ ), we have

$$\begin{aligned}
 & \mathbb{E}_{\mathbf{x} \sim q} [\hat{Z}_0[h]^2] \\
 &= \mathbb{E}_{\mathbf{x} \sim q} \left[ \left( \frac{2}{n} \sum_{i \in \mathcal{D}_1} w_*(x_i) (h(x_i) - \hat{h}_{\mathcal{D}_0}(x_i)) \right)^2 \right] \\
 &= \frac{4}{n^2} \mathbb{E}_{\mathbf{x}_{\mathcal{D}_0} \sim q} \left\{ \sum_{i \in \mathcal{D}_1} \mathbb{E}_{x_i \sim q} [w_*(x_i)^2 (h(x_i) - \hat{h}_{\mathcal{D}_0}(x_i))^2] \right. \\
 &\quad \left. + \sum_{i \neq j; i, j \in \mathcal{D}_1} \mathbb{E}_{x_i, x_j \sim q} [w_*(x_i) (h(x_i) - \hat{h}_{\mathcal{D}_0}(x_i)) w_*(x_j) (h(x_j) - \hat{h}_{\mathcal{D}_0}(x_j))] \right\} \\
 &= \frac{4}{n^2} \mathbb{E}_{\mathbf{x}_{\mathcal{D}_0} \sim q} \left\{ \sum_{i \in \mathcal{D}_1} \mathbb{E}_r [(h(x_i) - \hat{h}_{\mathcal{D}_0}(x_i))^2] + \sum_{i \neq j; i, j \in \mathcal{D}_1} \mathbb{E}_p [(h(x_i) - \hat{h}_{\mathcal{D}_0}(x_i)) (h(x_j) - \hat{h}_{\mathcal{D}_0}(x_j))] \right\} \\
 &= \frac{2}{n} \mathbb{E}_{\mathbf{x}_{\mathcal{D}_0} \sim q} \left\{ \int \frac{p(x)^2}{q(x)} (h(x) - \hat{h}_0(x))^2 dx \right\} \quad (\text{because } \mathbb{E}_p h = \mathbb{E}_p \hat{h} = 0) \\
 &\leq \frac{2M_3}{n} \mathbb{E}_{\mathbf{x}_{\mathcal{D}_0} \sim q} \left\{ \mathbb{E}_p [(h(x) - \hat{h}_0(x))^2] \right\} \quad (\text{because } p(x)/q(x) \leq M_3 \text{ by assumption}) \\
 &= \frac{2M_3}{n} \mathbb{E}_{\mathbf{x}_{\mathcal{D}_0} \sim q} \left\{ \sum_{\ell > L} \beta_\ell^2 + \sum_{\ell < L} (\beta_\ell - \hat{\beta}_{\ell,0})^2 \right\} \\
 &= \frac{2M_3}{n} \left\{ \sum_{\ell > L} \beta_\ell^2 + \sum_{\ell < L} \text{var}_{\mathbf{x}_{\mathcal{D}_0} \sim q} (\hat{\beta}_{\ell,0}) \right\} \quad (\text{because } \mathbb{E}_{\mathbf{x}_{\mathcal{D}_0} \sim q} [\hat{\beta}_{\ell,0}] = \beta_\ell) \\
 &= \frac{2M_3}{n} \left[ \sum_{\ell > L} \beta_\ell^2 + \frac{2}{n} \sum_{\ell < L} \text{var}_{x \sim q} [w_*(x) \phi_\ell(x) h(x)] \right].
 \end{aligned}$$

We can derive the same result for  $\hat{Z}_1[h]$  and hence

$$\begin{aligned}
 \mathbb{E}_{\mathbf{x} \sim q} [\hat{Z}[h]^2] &\leq \frac{1}{2} (\mathbb{E}_{\mathbf{x} \sim q} [\hat{Z}_0[h]^2] + \mathbb{E}_{\mathbf{x} \sim q} [\hat{Z}_1[h]^2]) \\
 &= \frac{2M_3}{n} \left[ \sum_{\ell > L} \beta_\ell^2 + \frac{2}{n} \sum_{\ell < L} \text{var}_{x \sim q} [w_*(x) \phi_\ell(x) h(x)] \right].
 \end{aligned}$$

Taking  $h(x) = \phi_{\ell'}(x)$  for which we have  $\beta_\ell = \mathbb{I}[\ell = \ell']$ , we get

$$\mathbb{E}_q [\hat{Z}[\phi_{\ell'}]^2] \leq \begin{cases} \frac{4M_3}{n^2} \sum_{\ell < L} \text{var}_{x \sim q} [w_*(x) \phi_\ell(x) \phi_{\ell'}(x)] & \text{if } \ell' \leq L \\ \frac{2M_3}{n} + \frac{4M_3}{n^2} \sum_{\ell < L} \text{var}_{x \sim q} [w_*(x) \phi_\ell(x) \phi_{\ell'}(x)] & \text{if } \ell' > L. \end{cases}$$

Define  $\rho_{\ell\ell'} = \text{var}_{\mathbf{x} \sim q}[w_*(x)\phi_\ell(x)\phi_{\ell'}(x)]$  and we have  $\rho_{\ell\ell'} \leq M$  by Assumption 2.4. We have

$$\begin{aligned}
 \mathbb{E}_{\mathbf{x} \sim q}[\mathbb{S}(\{x_i, w_i(\mathbf{x})\}, p)] &= \mathbb{E}_{\mathbf{x} \sim q}\left[\sum_{i,j=1}^n w_i(\mathbf{x})w_j(\mathbf{x})k_p(x_i, x_j)\right] \\
 &= \mathbb{E}_{\mathbf{x} \sim q}\left[\sum_{i,j=1}^n w_i(\mathbf{x})w_j(\mathbf{x})\sum_{\ell=1}^{\infty} \lambda_\ell \phi_\ell(x_i)\phi_\ell(x_j)\right] \\
 &= \sum_{\ell} \lambda_\ell \mathbb{E}_{\mathbf{x} \sim q}\left[\left(\sum_{i=1}^n w_i(\mathbf{x})\phi_\ell(x_i)\right)^2\right] \\
 &= \sum_{\ell} \lambda_\ell \mathbb{E}_{\mathbf{x} \sim q}[\hat{Z}[\phi_\ell]^2] \\
 &\leq \frac{2M_3}{n}\left[\sum_{\ell>L} \lambda_\ell + \frac{2}{n}\sum_{\ell=1}^{\infty} \lambda_\ell \sum_{\ell'<L} \rho_{\ell\ell'}\right] \\
 &\leq \frac{2}{n}\left[M_3 \sum_{\ell>L} \lambda_\ell + M_4 \frac{L}{n}\right],
 \end{aligned}$$

where  $M_4 = 2M_3 \max_{\ell'} \{\sum_{\ell} \lambda_\ell \rho_{\ell\ell'}\} \leq 2M_3 M \text{trace}(k_p)$ .  $\square$

### Step 3: Meeting the Non-negative and Normalization Constraint

The weights defined in (2.6) is not normalized to sum to one, and may also have negative values. To complete the proof, we define a set of new weights,

$$w_i^+(\mathbf{x}) = \frac{\max(0, w_i(\mathbf{x}))}{\sum_i \max(0, w_i(\mathbf{x}))}.$$

We need to give the bound for  $\mathbb{S}(\{x_i, w_i^+(\mathbf{x})\}, p)$  based on the bound of  $\mathcal{O}(\mathbb{S}(\{x_i, w_i(\mathbf{x})\}, p))$ . The key observation is that we have  $\sum_{i=1}^n w_i(\mathbf{x}) \xrightarrow{p} 1$  and  $w_i(\mathbf{x}) \geq 0$  with high probability for the weights given by in Lemma 2.6.

**Lemma 2.8.** *For the weights  $\{w_i(\mathbf{x})\}$  defined in Lemma 2.6, under Assumption 2.4, we have*

i). *When  $\mathbf{x} = \{x_i\}_{i=1}^n \sim q$ , we have*

$$\Pr[w_i(\mathbf{x}) < 0] \leq \exp\left(-\frac{n}{LM_2^2 M_3^2}\right), \quad \text{for } \forall i \leq n. \quad (3)$$

ii). *We have  $\mathbb{E}_{\mathbf{x} \sim q}[\sum_i w_i(\mathbf{x})] = 1$ . Assume  $L \geq 1$ , we have*

$$\Pr(S < 1 - t) \leq 2 \exp\left(-\frac{n}{L^2 M_s}\right) \quad \text{where} \quad M_s = M_3^2(M_2 M_3 + \sqrt{2})^2/4, \quad (4)$$

*Proof.* i). Recall that

$$w_i(\mathbf{x}) = \begin{cases} \frac{1}{n} w_*(x_i) - \frac{2}{n^2} \sum_{j \in \mathcal{D}_1} w_*(x_i) w_*(x_j) k_L(x_j, x_i), & \forall i \in \mathcal{D}_0 \\ \frac{1}{n} w_*(x_i) - \frac{2}{n^2} \sum_{j \in \mathcal{D}_0} w_*(x_i) w_*(x_j) k_L(x_j, x_i), & \forall i \in \mathcal{D}_1. \end{cases}$$

We just need to prove (3) for  $i \in \mathcal{D}_0$ . Note that

$$w_i(\mathbf{x}) = \frac{1}{n} w_*(x_i) [1 - T], \quad \text{where} \quad T = \frac{2}{n} \sum_{j \in \mathcal{D}_1} w_*(x_j) k_L(x_j, x_i).$$

Because  $\mathbb{E}[T \mid x_i] = \mathbb{E}_{\mathbf{x}' \sim q}[w_*(x') k_L(x', x_i)] = 0$  for  $\forall x$  and  $|w(x') k_L(x, x')| \leq LM_2 M_3$ ,  $\forall x, x' \in \mathcal{X}$ , using Hoeffding's inequality, we have

$$\Pr(w_i(\mathbf{x}) < 0) = \Pr(T > 1) \leq \exp\left(-\frac{n}{L^2 M_2^2 M_3^2}\right).$$

ii). Note that  $S \stackrel{\text{def}}{=} \sum_i w_i(\mathbf{x}) = S_1 + S_2$ ,

$$\text{where} \quad S_1 = \frac{1}{n} \sum_{i=1}^n w_*(x_i), \quad S_2 = -\frac{2}{n^2} \sum_{i \in \mathcal{D}_0} \sum_{j \in \mathcal{D}_1} w_*(x_i) w_*(x_j) k_L(x_i, x_j),$$

where the first term is the standard importance sampling weights and the second term comes from the control variate. It is easy to show that  $\mathbb{E}[S_1] = 1$  and  $\mathbb{E}[S_2] = 0$ , and hence  $\mathbb{E}[S] = 1$ . To prove the tail bound, note that for any  $t_1 + t_2 = t$ ,  $t_1, t_2 > 0$ , we have

$$\begin{aligned} \Pr(S < 1 - t) &\leq \Pr(S_1 < 1 - t_1) + \Pr(S_2 \leq t_2) \\ &\leq \exp\left(-\frac{2nt_1^2}{M_3^2}\right) + \exp\left(-\frac{4nt_2^2}{L^2 M_2^2 M_3^4}\right), \end{aligned}$$

where the bound for  $S_2$  uses the Hoeffding's inequality for two-sample U statistics [Hoeffding, 1963, Section 5b]. We take  $t_1 = \sqrt{2}t/(LM_2M_3 + \sqrt{2})$ , we have

$$\Pr(S < 1 - t) \leq 2 \exp\left(-\frac{4nt^2}{L^2 M_3^2 (M_2 M_3 + \sqrt{2}/L)^2}\right) \leq 2 \exp\left(-\frac{nt^2}{L^2 M_s}\right),$$

where  $M_s = M_3^2(M_2 M_3 + \sqrt{2})^2/4$  (we assume  $L \geq 1$ ).

□

**Lemma 2.9.** *Under Assumption 2.4, we have*

$$\mathbb{E}[\mathbb{S}(\{x_i, w_i^+(\mathbf{x})\}, p)] \leq \frac{1}{4} \mathbb{E}[\mathbb{S}(\{x_i, w_i(\mathbf{x})\}, p)] + M_f(n+2) \exp\left(-\frac{n}{L^2 M_0}\right),$$

where  $M_f = \text{trace}(k_p(x, x'))M_2$  and  $M_0 = \max(M_2^2 M_3, M_3^2(M_2 M_3 + \sqrt{2})^2)$ .

*Proof.* We use short notation  $f(\mathbf{w}^+) = \mathbb{S}(\{x_i, w_i^+(\mathbf{x})\}, p)$  for convenience. We have

$$|f(\mathbf{w}^+)| = \left| \sum_{\ell} \lambda_{\ell} \left( \sum_i w_i^+ \phi_{\ell}(x_i) \right)^2 \right| \leq \text{trace}(k_p(x, x')) M_2 \stackrel{\text{def}}{=} M_f.$$

Define  $\mathcal{E}_n$  to be the event that all  $w_i > 0$  and  $\sum_i w_i \geq 1/2$ , that is,  $\mathcal{E}_n = \{\sum_i w_i \geq 1/2, w_i \geq 0, \forall i \in [n]\}$ . We have from Lemma 2.8 that

$$\Pr(\bar{\mathcal{E}}_n) \leq n \exp\left(-\frac{n}{L^2 M_2^2 M_3}\right) + 2 \exp\left(-\frac{n}{4L^2 M_s}\right).$$

Note that under event  $\mathcal{E}_n$ , we have  $\mathbf{w} = \mathbf{w}^+$ . Therefore,

$$\begin{aligned} \mathbb{E}[f(\mathbf{w}^+)] &= \mathbb{E}[f(\mathbf{w}^+) | \mathcal{E}_n] \cdot \Pr[\mathcal{E}_n] + \mathbb{E}[f(\mathbf{w}^+) | \bar{\mathcal{E}}_n] \cdot \Pr[\bar{\mathcal{E}}_n] \\ &\leq \mathbb{E}[f(\mathbf{w}^+) | \mathcal{E}_n] \cdot \Pr[\mathcal{E}_n] + M_f \cdot \Pr[\bar{\mathcal{E}}_n] \\ &\leq \frac{1}{4} \mathbb{E}[f(\mathbf{w}) | \mathcal{E}_n] \cdot \Pr[\mathcal{E}_n] + M_f \cdot \Pr[\bar{\mathcal{E}}_n] \\ &\leq \frac{1}{4} \mathbb{E}[f(\mathbf{w})] + M_f \cdot \Pr[\bar{\mathcal{E}}_n] \\ &\leq \frac{1}{4} \mathbb{E}[f(\mathbf{w})] + M_f \cdot \left[ n \exp\left(-\frac{n}{L^2 M_2^2 M_3}\right) + 2 \exp\left(-\frac{n}{4L^2 M_s}\right) \right] \\ &\leq \frac{1}{4} \mathbb{E}[f(\mathbf{w})] + M_f(n+2) \exp\left(-\frac{n}{L^2 M_0}\right) \end{aligned}$$

□

### 3 Additional Empirical Results

Here we show in Figure 1 an additional empirical result when  $p(x)$  is a Gaussian mixture model shown in Figure 1(a) and  $\{x_i\}_{i=1}^n$  is generated by running  $n$  independent chains of MALA for 10 steps.



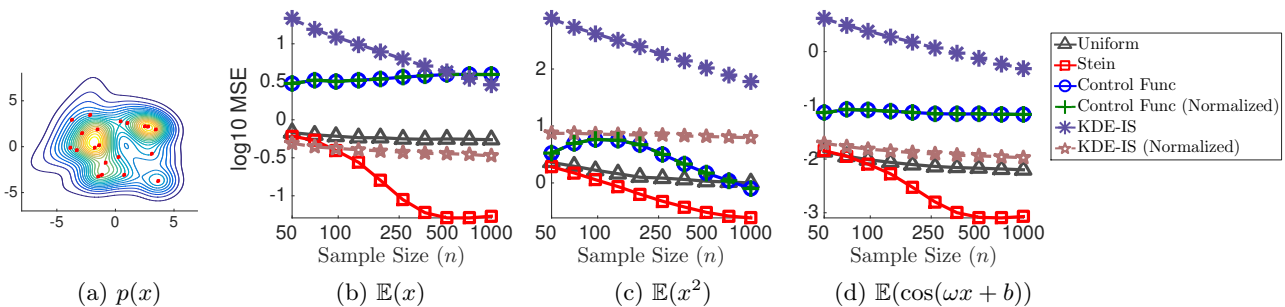

Figure 1: Gaussian Mixture Example. (a) The contour of the distribution  $p(x)$  that we use, and  $\{x_i\}_{i=1}^n$  is generated by running  $n$  independent MALA for 10 steps. (b) - (c) The MSE of the different weighting schemes for estimating  $\mathbb{E}(h(x))$ , where  $h(x)$  equals  $x$ ,  $x^2$ , and  $\cos(\omega x + b)$ , respectively. For  $h = \cos(\omega x + b)$  in (c), we draw  $\omega \sim \mathcal{N}(0, 1)$  and  $b \sim \text{Uniform}([0, 2\pi])$  and average the MSE over 20 random trials.

## References

- R. Morris, X. Descombes, and J. Zerubia. The Ising/Potts model is not well suited to segmentation tasks. In *Digital Signal Processing Workshop Proceedings, 1996.*, IEEE, pages 263–266. IEEE, 1996.
- M. Welling and Y. W. Teh. Bayesian learning via stochastic gradient Langevin dynamics. In *ICML*, 2011.
- P. Alquier, N. Friel, R. Everitt, and A. Boland. Noisy Monte Carlo: Convergence of markov chains with approximate transition kernels. *Statistics and Computing*, 26(1-2):29–47, 2016.
- A. O’Hagan. Monte carlo is fundamentally unsound. *Journal of the Royal Statistical Society. Series D (The Statistician)*, 36(2/3):247–249, 1987.
- M. Henmi, R. Yoshida, and S. Eguchi. Importance sampling via the estimated sampler. *Biometrika*, 94(4): 985–991, 2007.
- B. Delyon and F. Portier. Integral approximation by kernel smoothing. *arXiv preprint arXiv:1409.0733*, 2014.
- D. J. Rezende and S. Mohamed. Variational inference with normalizing flows. In *ICML*, 2015.
- B. Efron. Bayesian inference and the parametric bootstrap. *The annals of applied statistics*, 6(4):1971, 2012.
- T. Hazan, S. Maji, and T. Jaakkola. On sampling from the gibbs distribution with random maximum a-posteriori perturbations. In *NIPS*, pages 1268–1276, 2013.
- G. Papandreou and A. L. Yuille. Perturb-and-map random fields: Using discrete optimization to learn and sample from energy models. In *ICCV*, pages 193–200. IEEE, 2011.
- Q. Liu, J. W. Fisher III, and A. T. Ihler. Probabilistic variational bounds for graphical models. In *NIPS*, pages 1432–1440, 2015.
- C. Wang, X. Chen, A. J. Smola, and E. P. Xing. Variance reduction for stochastic gradient optimization. In *Advances in Neural Information Processing Systems*, pages 181–189, 2013.
- R. Ranganath, S. Gerrish, and D. M. Blei. Black box variational inference. In *AISTATS*, pages 814–822, 2014.
- M. Sugiyama, S. Nakajima, H. Kashima, P. V. Buenau, and M. Kawanabe. Direct importance estimation with model selection and its application to covariate shift adaptation. In *NIPS*, 2008.
- L. Li, R. Munos, and C. Szepesvári. Toward minimax off-policy value estimation. In *AISTATS*, 2015.
- P. Zhao and T. Zhang. Stochastic optimization with importance sampling. *ICML*, 2015.
- C. J. Oates, M. Girolami, and N. Chopin. Control functionals for Monte Carlo integration. *Journal of the Royal Statistical Society, Series B*, 2017.
- K. Chwialkowski, H. Strathmann, and A. Gretton. A kernel test of goodness of fit. In *ICML*, 2016.
- Q. Liu, J. D. Lee, and M. I. Jordan. A kernelized stein discrepancy for goodness-of-fit tests and model evaluation. In *ICML*, 2016.
- F.-X. Briol, C. Oates, M. Girolami, M. A. Osborne, D. Sejdinovic, et al. Probabilistic integration: A role for statisticians in numerical analysis? *arXiv preprint http://arxiv.org/abs/1512.00933*, 2015a.

- F.-X. Briol, C. Oates, M. Girolami, and M. A. Osborne. Frank-Wolfe Bayesian Quadrature: Probabilistic integration with theoretical guarantees. In *NIPS*, 2015b.
- A. O’Hagan. Bayes–Hermite quadrature. *Journal of statistical planning and inference*, 29(3):245–260, 1991.
- Z. Ghahramani and C. E. Rasmussen. Bayesian Monte Carlo. In *NIPS*, 2002.
- M. Sugiyama and M. Kawanabe. *Machine learning in non-stationary environments: Introduction to covariate shift adaptation*. MIT Press, 2012.
- L. Martino, V. Elvira, D. Luengo, and J. Corander. Layered adaptive importance sampling. *Statistics and Computing*, pages 1–25.
- Z. I. Botev, P. L’Ecuyer, and B. Tuffin. Markov chain importance sampling with applications to rare event probability estimation. *Statistics and Computing*, 23(2):271–285, 2013.
- F. Beaujean and A. Caldwell. Initializing adaptive importance sampling with markov chains. *arXiv preprint arXiv:1304.7808*, 2013.
- X. Yuan, Z. Lu, C. Zhou, and Z. Yue. A novel adaptive importance sampling algorithm based on markov chain and low-discrepancy sequence. *Aerospace Science and Technology*, 29(1):253–261, 2013.
- A. Smith, A. Doucet, N. de Freitas, and N. Gordon. *Sequential Monte Carlo Methods in Practice*. Springer Science & Business Media, 2013.
- C. Robert and G. Casella. *Monte Carlo statistical methods*. Springer Science & Business Media, 2013.
- R. M. Neal. Annealed importance sampling. *Statistics and Computing*, 11(2):125–139, 2001.
- Y. Chen, M. Welling, and A. Smola. Super-samples from kernel herding. In *UAI*, 2010.
- F. Bach. On the equivalence between quadrature rules and random features. *arXiv preprint arXiv:1502.06800*, 2015.
- F. Huszár and D. Duvenaud. Optimally-weighted Herding is Bayesian quadrature. In *UAI*, 2012.
- H. Niederreiter. *Quasi-Monte Carlo Methods*. Wiley Online Library, 2010.
- S. N. MacEachern, M. Clyde, and J. S. Liu. Sequential importance sampling for nonparametric Bayes models: The next generation. *Canadian Journal of Statistics*, 27(2):251–267, 1999.
- M. J. Wainwright and M. I. Jordan. Graphical models, exponential families, and variational inference. *Foundations and Trends® in Machine Learning*, 1(1-2):1–305, 2008.
- L. Breiman. Better subset regression using the nonnegative garrote. *Technometrics*, 37(4):373–384, 1995.
- B. L. Nelson. On control variate estimators. *Computers & Operations Research*, 14(3):219–225, 1987.
- J. S. Liu. *Monte Carlo strategies in scientific computing*. Springer Science & Business Media, 2008.
- A. Gretton, K. M. Borgwardt, M. J. Rasch, B. Schölkopf, and A. Smola. A kernel two-sample test. *The Journal of Machine Learning Research*, 13(1):723–773, 2012.
- Y. W. Teh, A. H. Thiery, and S. J. Vollmer. Consistency and fluctuations for stochastic gradient langevin dynamics. *Journal of Machine Learning Research*, 17, 2016.
- K. Bache and M. Lichman. UCI machine learning repository, 2013. URL <http://archive.ics.uci.edu/ml>.
- R. Collobert, S. Bengio, and Y. Bengio. A parallel mixture of SVMs for very large scale problems. *Neural computation*, 14(5):1105–1114, 2002.
- M. D. Hoffman and A. Gelman. The no-u-turn sampler: adaptively setting path lengths in hamiltonian monte carlo. *Journal of Machine Learning Research*, 15(1):1593–1623, 2014.
- J. Lee. *U-statistics: Theory and Practice*. CRC Press, 1990.
- W. Hoeffding. Probability inequalities for sums of bounded random variables. *Journal of the American statistical association*, 58(301):13–30, 1963.
